# Supplementary material for: Self-supporting Structure of Bird Nests
Source: arXiv:2401.05371 source file (2023-12-15)
Supplement: Supplementary file 1 [file Appendix.pdf]

# Appendix 1. String Entanglement

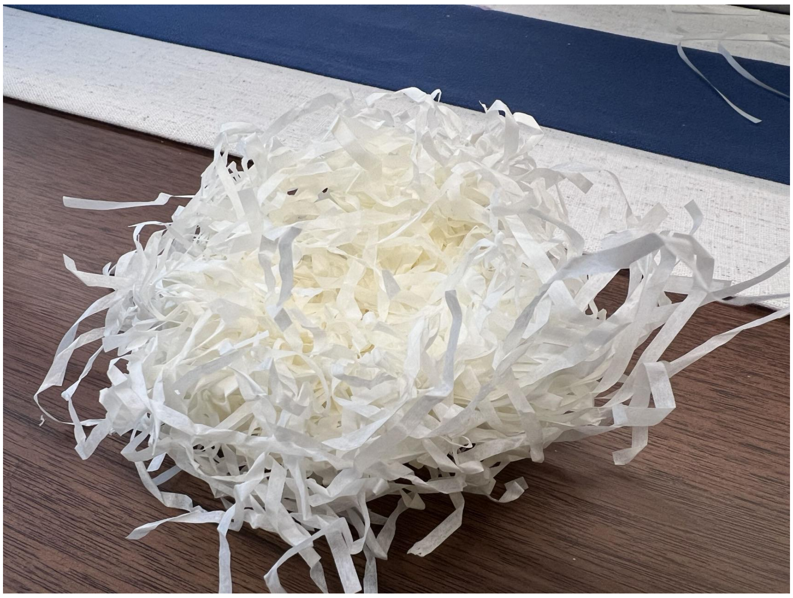

As an attempt to learn how nests form and how they can stay stable, we, as a team, tried to describe the stability of the nests using the term “Entanglement degree”. The entanglement degree of a nest is defined by whether the pieces of the nests would be taken out when the nests are well constructed and connected. In other words, the higher the entanglement degree, the more secure and resilient the nest is likely to be. To quantify the entanglement degree, one could consider factors such as the number of connections between the pieces, the strength of those connections, the distribution of forces within the nest, and the overall shape and symmetry of the structure. A well-constructed nest with a high entanglement degree should be able to withstand external disturbances and remain stable.

Procedure

Step 1

Prepare 100 paper strings.

Step 2

Put the string together, try to make them into a nest by using different strategies, by either kneading them up or simply put them together.

Step 3

After the nest is constructed, randomly pull one string from the whole nest. Let the string put force the gravitational force from the nest. In this case, if the nest falls down from the string, it would be counted as a failure. If the nest does not fall down, it would be counted as a success.

Step 4

Use the number of success to divide the total amount of strings picked. The ratio would be recorded as the entanglement degree.

Step 5

Repeat the above process for 2 or 3 other amount of strings. Pick some amount of strings in response to the amount of strings in total. Then, calculate the corresponding entanglement degree, and compare the results.

Result

| | | | |
|---|---|---|---|
| 1 | 1 | 26 | 1 |
| 2 | 1 | 27 | 1 |
| 3 | 0 | 28 | 0 |
| 4 | 1 | 29 | 1 |
| 5 | 1 | 30 | 1 |
| 6 | 0 | 31 | 0 |
| 7 | 1 | 32 | 1 |
| 8 | 0 | 33 | 0 |
| 9 | 0 | 34 | 1 |
| 10 | 0 | 35 | 1 |
| 11 | 0 | 36 | 1 |
| 12 | 1 | 37 | 1 |
| 13 | 1 | 38 | 1 |
| 14 | 1 | 39 | 0 |
| 15 | 1 | 40 | 1 |
| 16 | 1 | 41 | 1 |
| 17 | 0 | 42 | 0 |
| 18 | 1 | 43 | 0 |
| 19 | 1 | 44 | 0 |
| 20 | 1 | 45 | 1 |
| 21 | 1 | 46 | 0 |
| 22 | 1 | 47 | 1 |
| 23 | 1 | 48 | 0 |
| 24 | 1 | 49 | 0 |
| 25 | 0 | 50 | 1 |

The entanglement degree of 50 strings would be 0.64.

| | |
|---|---|
| 1 | 1 |
| 2 | 1 |
| 3 | 1 |
| 4 | 1 |
| 5 | 1 |
| 6 | 1 |
| 7 | 1 |
| 8 | 1 |
| 9 | 1 |
| 10 | 1 |

The entanglement degree of 20 strings would be 1, meaning that it is always stable, without any destruction.

| | | | |
|---|---|---|---|
| 1 | 0 | 51 | 0 |

| | | | |
|---|---|---|---|
| 2 | 1 | 52 | 0 |
| 3 | 0 | 53 | 0 |
| 4 | 1 | 54 | 1 |
| 5 | 1 | 55 | 1 |
| 6 | 1 | 56 | 1 |
| 7 | 0 | 57 | 1 |
| 8 | 0 | 58 | 0 |
| 9 | 0 | 59 | 0 |
| 10 | 0 | 60 | 1 |
| 11 | 1 | 61 | 0 |
| 12 | 1 | 62 | 0 |
| 13 | 0 | 63 | 0 |
| 14 | 0 | 64 | 0 |
| 15 | 0 | 65 | 0 |
| 16 | 1 | 66 | 0 |
| 17 | 0 | 67 | 0 |
| 18 | 0 | 68 | 0 |
| 19 | 0 | 69 | 0 |
| 20 | 0 | 70 | 1 |
| 21 | 0 | 71 | 0 |
| 22 | 1 | 72 | 0 |
| 23 | 0 | 73 | 0 |
| 24 | 1 | 74 | 0 |
| 25 | 0 | 75 | 1 |
| 26 | 1 | 76 | 0 |
| 27 | 0 | 77 | 1 |
| 28 | 1 | 78 | 1 |
| 29 | 1 | 79 | 1 |
| 30 | 1 | 80 | 1 |
| 31 | 0 | 81 | 1 |
| 32 | 1 | 82 | 1 |
| 33 | 1 | 83 | 1 |
| 34 | 1 | 84 | 1 |
| 35 | 0 | 85 | 0 |
| 36 | 0 | 86 | 1 |
| 37 | 0 | 87 | 1 |
| 38 | 1 | 88 | 1 |
| 39 | 1 | 89 | 0 |
| 40 | 1 | 90 | 1 |
| 41 | 0 | 91 | 1 |
| 42 | 0 | 92 | 1 |
| 43 | 1 | 93 | 0 |
| 44 | 1 | 94 | 0 |
| 45 | 1 | 95 | 0 |

| | | | |
|---|---|---|---|
| 46 | 1 | 96 | 1 |
| 47 | 1 | 97 | 0 |
| 48 | 0 | 98 | 1 |
| 49 | 1 | 99 | 0 |
| 50 | 1 | 100 | 1 |

The entanglement for 200 strings would be 0.5.

As we can see from the results, as the amount of strings increases, the value of entanglement degree would decrease. This can lead to our hypothesis that the degree actually depends on a limit. If the total amount of weight succeeds the maximum amount of connection between strings, the degree would decrease. Otherwise, the value would probably stay constant, and would not vary significantly.

Probability of forming the structure:

# Appendix 2. Random Packing of Sticks

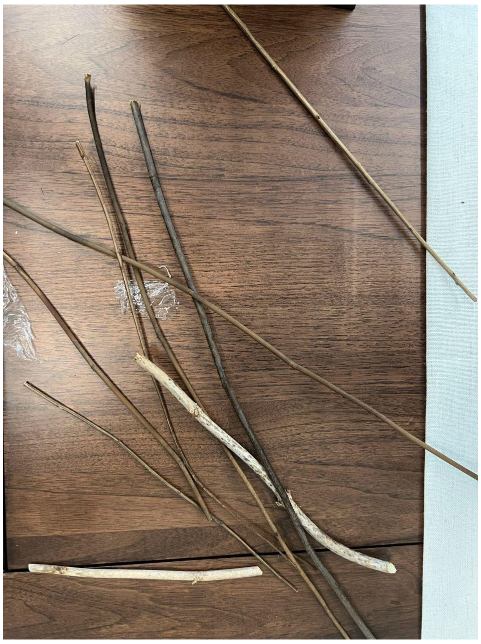

Procedure:
Step 1: Prepare 5 wooden sticks.
Step 2: Hold them up in a pile.
Step 3: Release them.
Step 4: Wait until the result is stable.
Step 5: Check if there exist the structure
Step 6: Repeat step 1-5 until there is the structure.

| | | | | | | | |
|---|---|---|---|---|---|---|---|
| 1 | 0 | 95 | 0 | 48 | 0 | 142 | 0 |
| 2 | 0 | 96 | 0 | 49 | 0 | 143 | 0 |
| 3 | 0 | 97 | 0 | 50 | 0 | 144 | 0 |
| 4 | 0 | 98 | 0 | 51 | 0 | 145 | 0 |
| 5 | 0 | 99 | 0 | 52 | 0 | 146 | 0 |
| 6 | 0 | 100 | 0 | 53 | 0 | 147 | 0 |
| 7 | 0 | 101 | 0 | 54 | 0 | 148 | 0 |
| 8 | 0 | 102 | 0 | 55 | 0 | 149 | 0 |
| 9 | 0 | 103 | 0 | 56 | 0 | 150 | 0 |
| 10 | 0 | 104 | 0 | 57 | 0 | 151 | 0 |
| 11 | 0 | 105 | 0 | 58 | 0 | 152 | 0 |
| 12 | 0 | 106 | 0 | 59 | 0 | 153 | 0 |
| 13 | 0 | 107 | 0 | 60 | 0 | 154 | 0 |
| 14 | 0 | 108 | 0 | 61 | 0 | 155 | 0 |
| 15 | 0 | 109 | 0 | 62 | 0 | 156 | 0 |
| 16 | 0 | 110 | 0 | 63 | 0 | 157 | 0 |
| 17 | 0 | 111 | 0 | 64 | 0 | 158 | 0 |
| 18 | 0 | 112 | 0 | 65 | 0 | 159 | 0 |
| 19 | 0 | 113 | 0 | 66 | 0 | 160 | 0 |
| 20 | 0 | 114 | 0 | 67 | 0 | 161 | 0 |

| | | | | | | | |
|---|---|---|---|---|---|---|---|
| 21 | 0 | 115 | 0 | 68 | 0 | 162 | 0 |
| 22 | 0 | 116 | 0 | 69 | 0 | 163 | 0 |
| 23 | 0 | 117 | 0 | 70 | 0 | 164 | 0 |
| 24 | 0 | 118 | 0 | 71 | 0 | 165 | 0 |
| 25 | 0 | 119 | 0 | 72 | 0 | 166 | 0 |
| 26 | 0 | 120 | 0 | 73 | 0 | 167 | 0 |
| 27 | 0 | 121 | 0 | 74 | 0 | 168 | 0 |
| 28 | 0 | 122 | 0 | 75 | 0 | 169 | 0 |
| 29 | 0 | 123 | 0 | 76 | 0 | 170 | 0 |
| 30 | 0 | 124 | 0 | 77 | 0 | 171 | 0 |
| 31 | 0 | 125 | 0 | 78 | 0 | 172 | 0 |
| 32 | 0 | 126 | 0 | 79 | 0 | 173 | 0 |
| 33 | 0 | 127 | 0 | 80 | 0 | 174 | 0 |
| 34 | 0 | 128 | 0 | 81 | 0 | 175 | 0 |
| 35 | 0 | 129 | 0 | 82 | 0 | 176 | 0 |
| 36 | 0 | 130 | 0 | 83 | 0 | 177 | 0 |
| 37 | 0 | 131 | 0 | 84 | 0 | 178 | 0 |
| 38 | 0 | 132 | 0 | 85 | 0 | 179 | 0 |
| 39 | 0 | 133 | 0 | 86 | 0 | 180 | 0 |
| 40 | 0 | 134 | 0 | 87 | 0 | 181 | 0 |
| 41 | 0 | 135 | 0 | 88 | 0 | 182 | 0 |
| 42 | 0 | 136 | 0 | 89 | 0 | 183 | 0 |
| 43 | 0 | 137 | 0 | 90 | 0 | 184 | 0 |
| 44 | 0 | 138 | 0 | 91 | 0 | 185 | 0 |
| 45 | 0 | 139 | 0 | 92 | 0 | 186 | 0 |
| 46 | 0 | 140 | 0 | 93 | 0 | 187 | 0 |
| 47 | 0 | 141 | 0 | 94 | 0 | 188 | 1 |

For 5 sticks, it takes 188 trials

Procedure:
Step 1: Prepare 6 wooden sticks.
Step 2: Hold them up in a pile.
Step 3: Release them.
Step 4: Wait until the result is stable.
Step 5: Check if there exist the structure
Step 6: Repeat step 1-5 until there is the structure.

| | | | |
|---|---|---|---|
| 1 | 0 | 48 | 0 |
| 2 | 0 | 49 | 0 |
| 3 | 0 | 50 | 0 |
| 4 | 0 | 51 | 0 |
| 5 | 0 | 52 | 0 |
| 6 | 0 | 53 | 0 |
| 7 | 0 | 54 | 0 |

| | | | |
|---|---|---|---|
| 8 | 0 | 55 | 0 |
| 9 | 0 | 56 | 0 |
| 10 | 0 | 57 | 0 |
| 11 | 0 | 58 | 0 |
| 12 | 0 | 59 | 0 |
| 13 | 0 | 60 | 0 |
| 14 | 0 | 61 | 0 |
| 15 | 0 | 62 | 0 |
| 16 | 0 | 63 | 0 |
| 17 | 0 | 64 | 0 |
| 18 | 0 | 65 | 0 |
| 19 | 0 | 66 | 0 |
| 20 | 0 | 67 | 0 |
| 21 | 0 | 68 | 0 |
| 22 | 0 | 69 | 0 |
| 23 | 0 | 70 | 0 |
| 24 | 0 | 71 | 0 |
| 25 | 0 | 72 | 0 |
| 26 | 0 | 73 | 0 |
| 27 | 0 | 74 | 0 |
| 28 | 0 | 75 | 0 |
| 29 | 0 | 76 | 0 |
| 30 | 0 | 77 | 0 |
| 31 | 0 | 78 | 0 |
| 32 | 0 | 79 | 0 |
| 33 | 0 | 80 | 0 |
| 34 | 0 | 81 | 0 |
| 35 | 0 | 82 | 0 |
| 36 | 0 | 83 | 0 |
| 37 | 0 | 84 | 0 |
| 38 | 0 | 85 | 0 |
| 39 | 0 | 86 | 0 |
| 40 | 0 | 87 | 0 |
| 41 | 0 | 88 | 0 |
| 42 | 0 | 89 | 0 |
| 43 | 0 | 90 | 0 |
| 44 | 0 | 91 | 0 |
| 45 | 0 | 92 | 0 |
| 46 | 0 | 93 | 0 |
| 47 | 0 | 94 | 1 |

For 6 sticks, it takes 94 trials

Procedure:

Step 1: Prepare 7 wooden sticks.
Step 2: Hold them up in a pile.
Step 3: Release them.
Step 4: Wait until the result is stable.
Step 5: Check if there exist the structure
Step 6: Repeat step 1-5 until there is the structure.

| | | | |
|---|---|---|---|
| 1 | 0 | 37 | 0 |
| 2 | 0 | 38 | 0 |
| 3 | 0 | 39 | 0 |
| 4 | 0 | 40 | 0 |
| 5 | 0 | 41 | 0 |
| 6 | 0 | 42 | 0 |
| 7 | 0 | 43 | 0 |
| 8 | 0 | 44 | 0 |
| 9 | 0 | 45 | 0 |
| 10 | 0 | 46 | 0 |
| 11 | 0 | 47 | 0 |
| 12 | 0 | 48 | 0 |
| 13 | 0 | 49 | 0 |
| 14 | 0 | 50 | 0 |
| 15 | 0 | 51 | 0 |
| 16 | 0 | 52 | 0 |
| 17 | 0 | 53 | 0 |
| 18 | 0 | 54 | 0 |
| 19 | 0 | 55 | 0 |
| 20 | 0 | 56 | 0 |
| 21 | 0 | 57 | 0 |
| 22 | 0 | 58 | 0 |
| 23 | 0 | 59 | 0 |
| 24 | 0 | 60 | 0 |
| 25 | 0 | 61 | 0 |
| 26 | 0 | 62 | 0 |
| 27 | 0 | 63 | 0 |
| 28 | 0 | 64 | 0 |
| 29 | 0 | 65 | 0 |
| 30 | 0 | 66 | 0 |
| 31 | 0 | 67 | 0 |
| 32 | 0 | 68 | 0 |
| 33 | 0 | 69 | 0 |
| 34 | 0 | 70 | 0 |
| 35 | 0 | 71 | 0 |
| 36 | 0 | 72 | 1 |

For 7 sticks, it takes 72 trials.

From the above data, it’s not hard to tell that as the number of sticks increases, the trails that takes to complete the structure is decreasing, probably because as the number of sticks increases, there’s more chances that a structure can be done. Relating back to bird nests, as the number of sticks is much more than 5,6 or 7, not to mention that bird nest are not being constructed under the environment of our lab, plane ground, yet complicated tree branches.

# Appendix 3. How to Determine the Height of a Rods Structures

We want to experimentally verify our theoretical prediction of height.

| d1 | d2 | h | theoretical |
|---|---|---|---|
| 6 | 1 | 0 | 0 |
| 6 | 3 | 0 | 0 |
| 6 | 5 | 4.3 | 4.8 |
| 6 | 7 | 3.3 | 3.428571 |
| 6 | 9 | 2.5 | 2.666667 |
| 6 | 11 | 2 | 2.181818 |
| 6 | 13 | 1.7 | 1.846154 |
| 6 | 15 | 1.5 | 1.6 |
| 6 | 17 | 1.3 | 1.411765 |
| 6 | 19 | 1.2 | 1.263158 |
| 6 | 21 | 1.1 | 1.142857 |

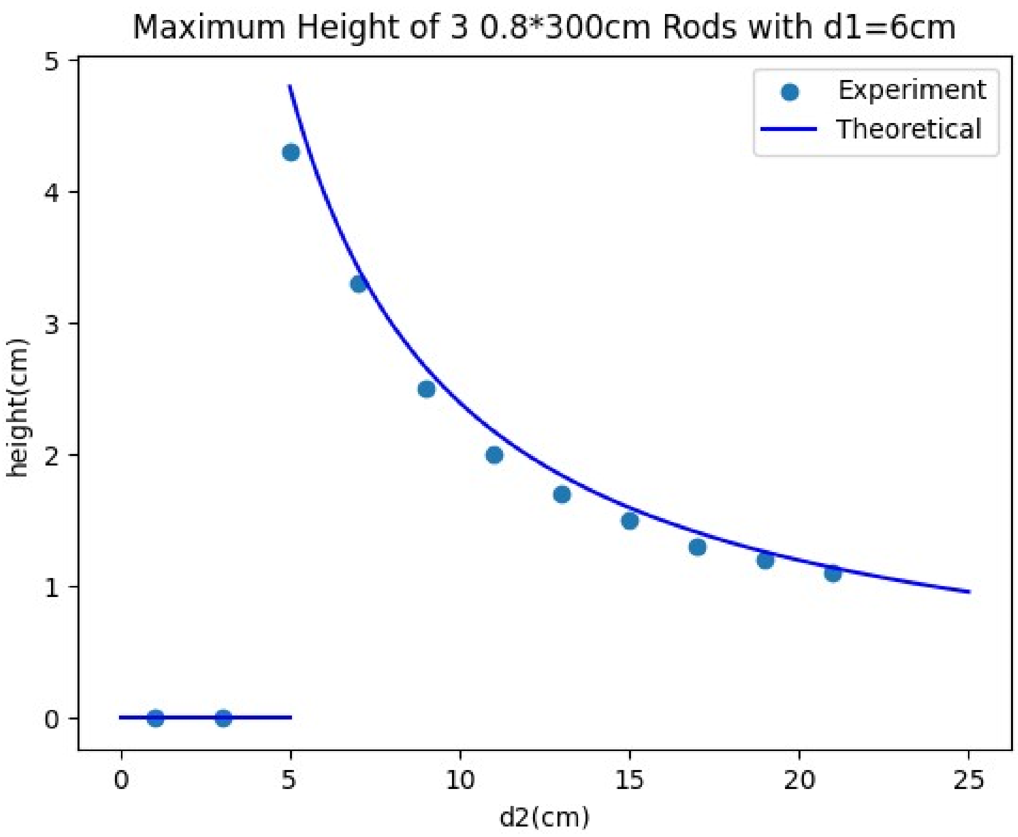
Maximum Height of 3 0.8*300cm Rods with d1=6cm
Experiment
Theoretical
height(cm)
d2(cm)
0
1
2
3
4
5
0
5
10
15
20
25

# Appendix 4.1 Not so Successful Equipments

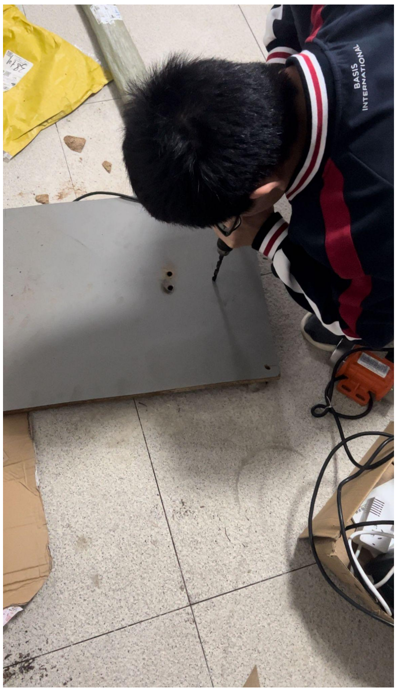

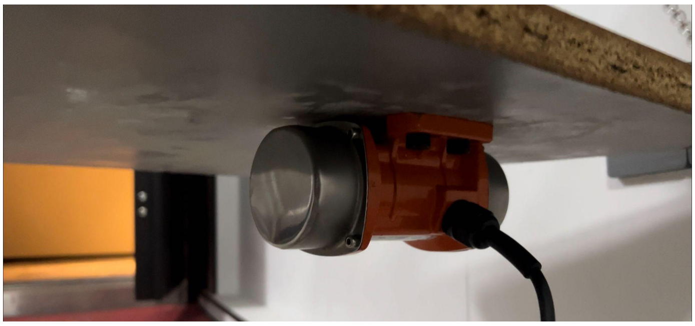

Initially, we tried to construct our own test bench by nailing a vibrator onto a wooden board, but the amplitude is too big for our structure, and the resonance of the system is unpredictable. Later, we purchased a more stable test bench online (much gratitude for Mark Xu's mom's support), and we used it for all the vibration experiments.

# Appendix 4.2 A not so Successful Way to Measure Amplitude

The purchased test bench displays frequency but not amplitude, and the amplitude may vary for each temperature and each weight configuration, so we first tried to measure amplitude through an optical lever.

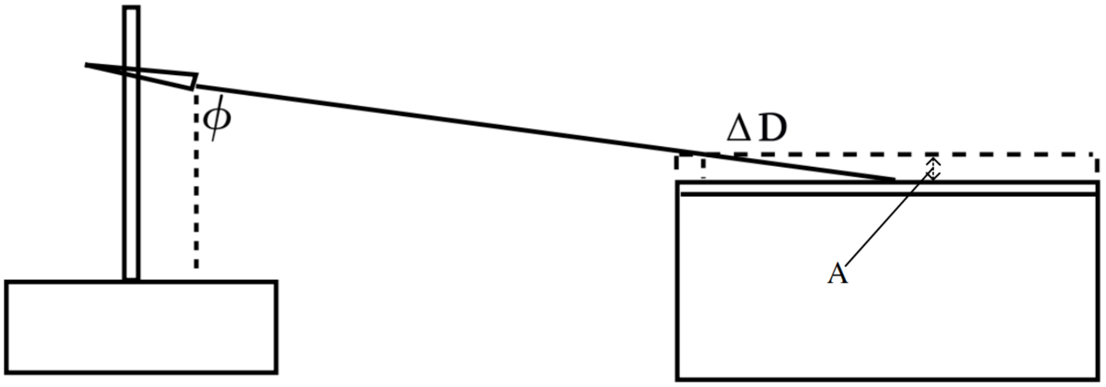


*A=Delta D/Phi*

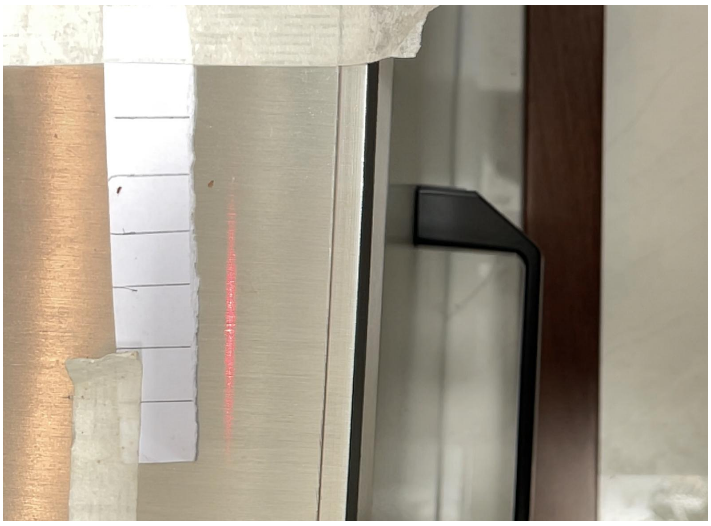

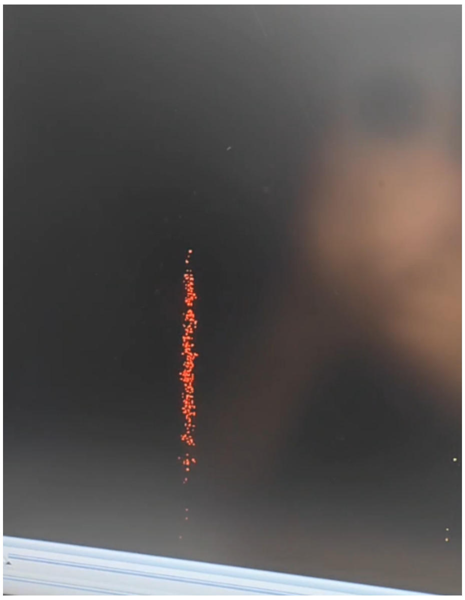

We recorded the movement of the light spot and analyze in tracker, but the magnification ratio is not big enough for us to make an accurate measurement, so we later purchased the vibrometer (much thanks to Mark Xu's mom) that conveniently and accurately measures amplitudes.

# Appendix 5. Other Materials

We uploaded videos and data tables to the Yau Awards official website.
Please refer to the attachments.

List of videos:

1. Vibration under Weight Experiment
2. Using Optical Lever to Measure Amplitude
3. Structures with d2=5 are very unstable
4. Vibration with no Weight Experiment
